# Supplementary material for: Wrinkle Mediated Phase Transitions in In$_2$Se$_3$
Source: arXiv:2507.16706 ancillary file (2025-07-22)
Supplement: Supplementary file 1 [file In2Se3_SupplementaryInfo_InitialSubmission-compressed.pdf]

## Supplementary Information for “Wrinkle Mediated Phase Transitions In<sub>2</sub>Se<sub>3</sub>”

Joseph L. Spellberg,<sup>1,2,\*</sup> Lina Kodaimati,<sup>2,\*</sup> Atreyie Ghosh,<sup>1</sup> Prakriti P. Joshi,<sup>3</sup> and Sarah B. King<sup>1,2,†</sup>

<sup>1</sup>*James Franck Institute, University of Chicago, Chicago, IL 60637, USA*

<sup>2</sup>*Department of Chemistry, University of Chicago, Chicago, IL 60637, USA*

<sup>3</sup>*Department of Physical Chemistry, Fritz-Haber-Institut der Max-Planck-Gesellschaft, Berlin 14195, Germany*

(Dated: July 21, 2025)

---

\* These two authors contributed equally.

† sbking@uchicago.edu; <http://kinglab.uchicago.edu>

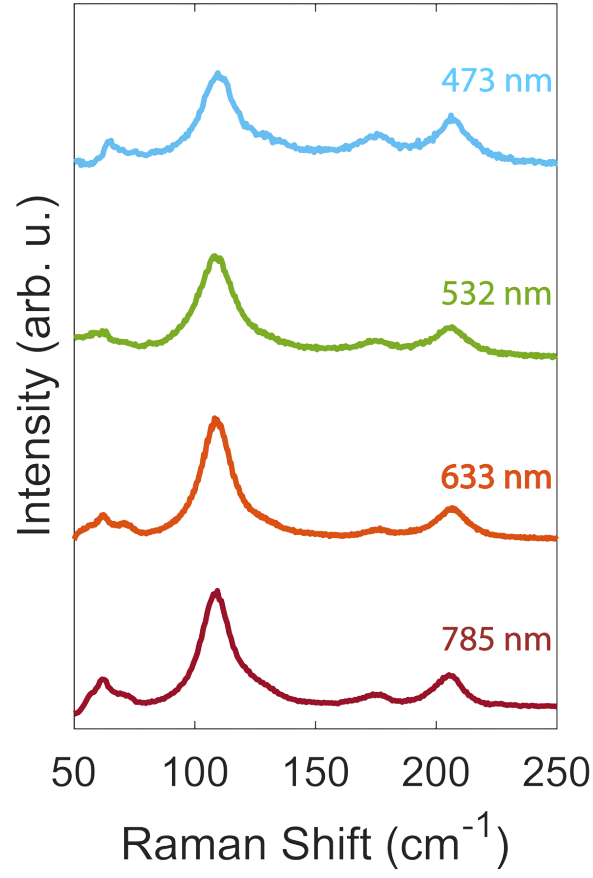

FIG. S1. Raman spectra collected on a  $\beta'$ -In<sub>2</sub>Se<sub>3</sub> flake with various excitation wavelengths.

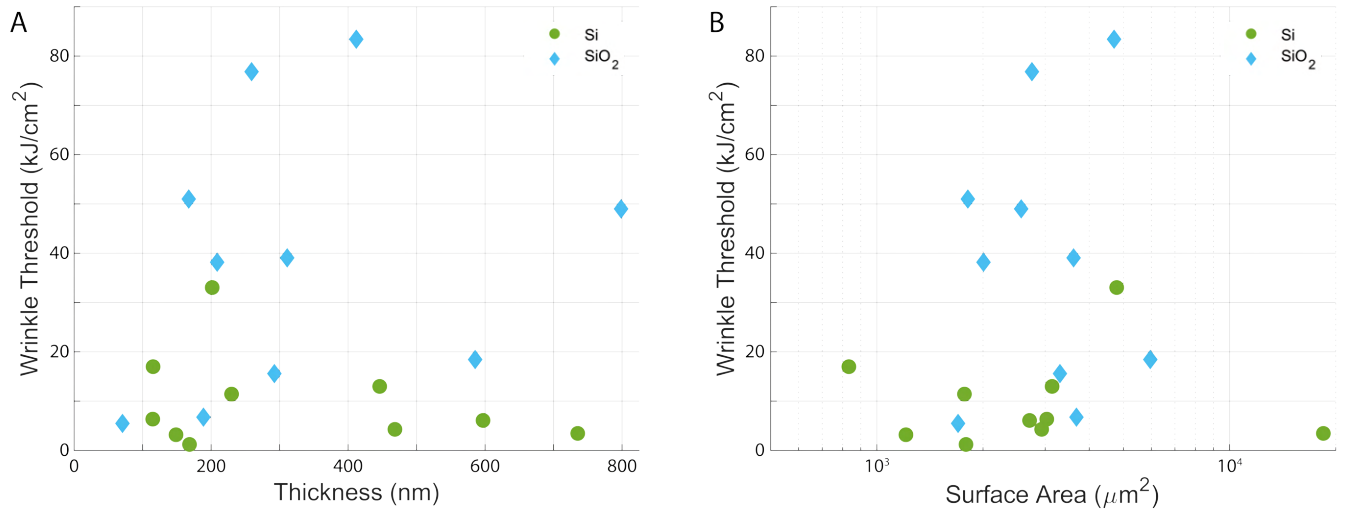

FIG. S2. Wrinkling threshold vs. (A) flake thickness and (B) flake surface area for flakes on Si with native oxide (green circles) and 100 nm thermal oxide SiO<sub>2</sub> (blue diamonds) substrates.

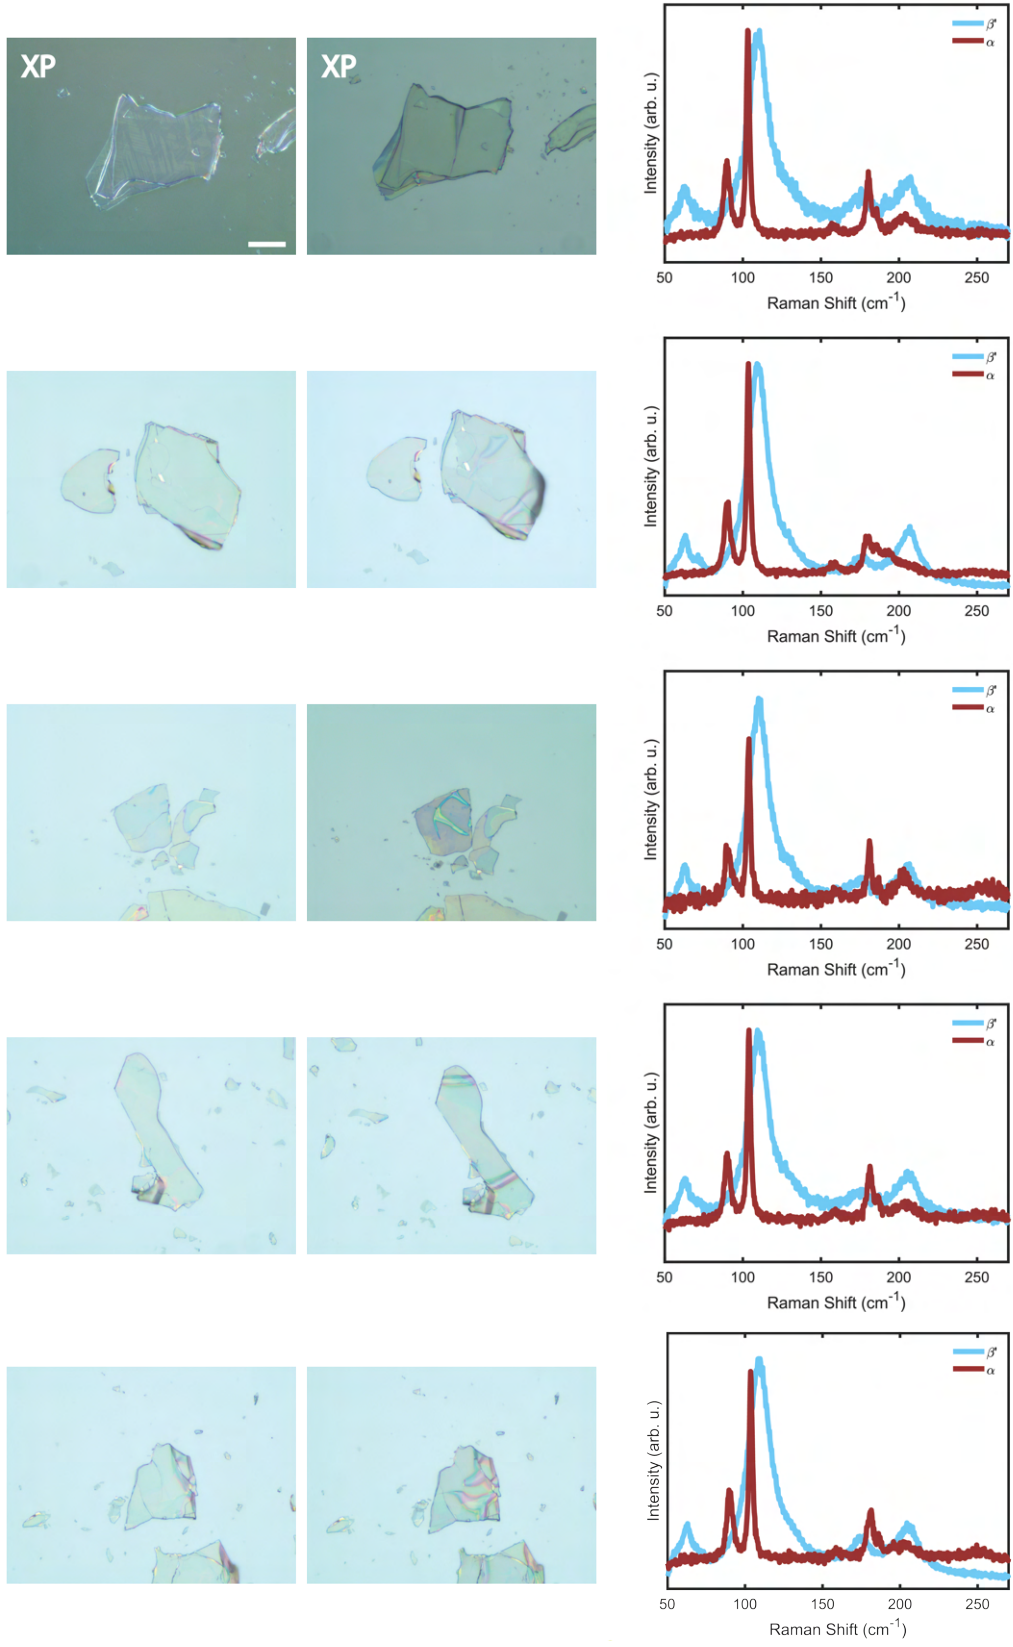

FIG. S3. Optical images and Raman spectra of flakes on Si substrate before and after wrinkling phase transition. Cross-polarized images where domain contrast can be observed are indicated with XP. Scale bars: 20  $\mu\text{m}$ .

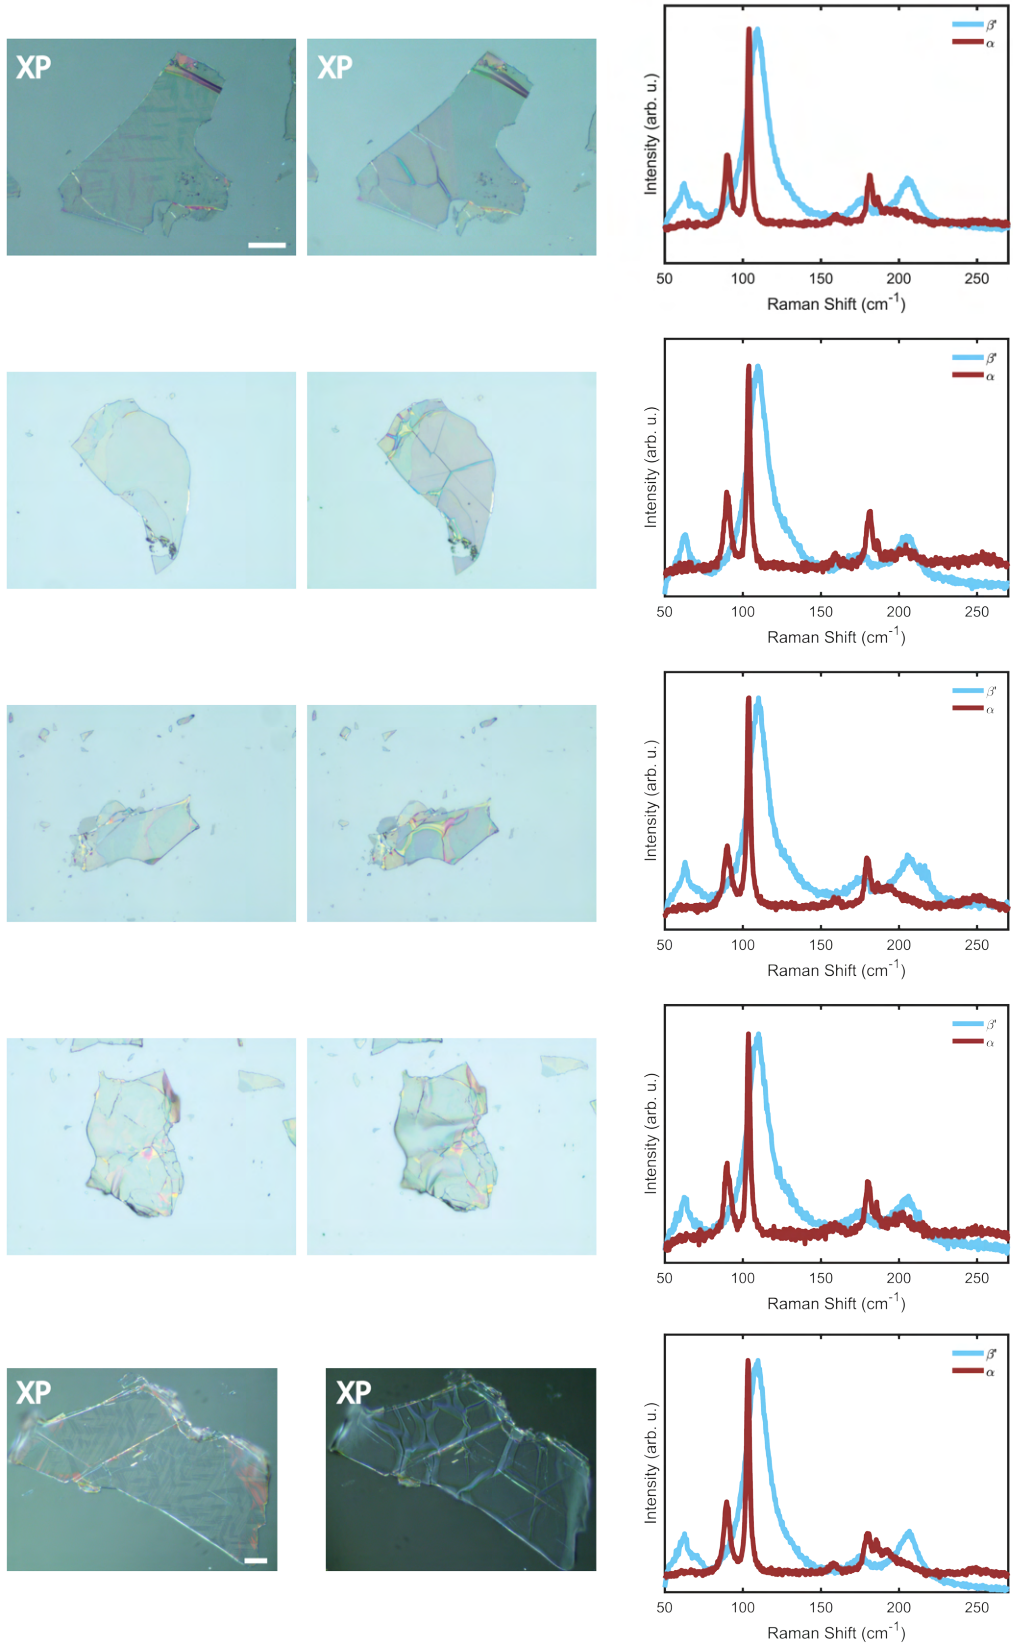

FIG. S4. Additional optical images and Raman spectra of flakes on Si substrate before and after wrinkling phase transition. Cross-polarized images where domain contrast can be observed are indicated with XP. Scale bars: 20  $\mu\text{m}$ .

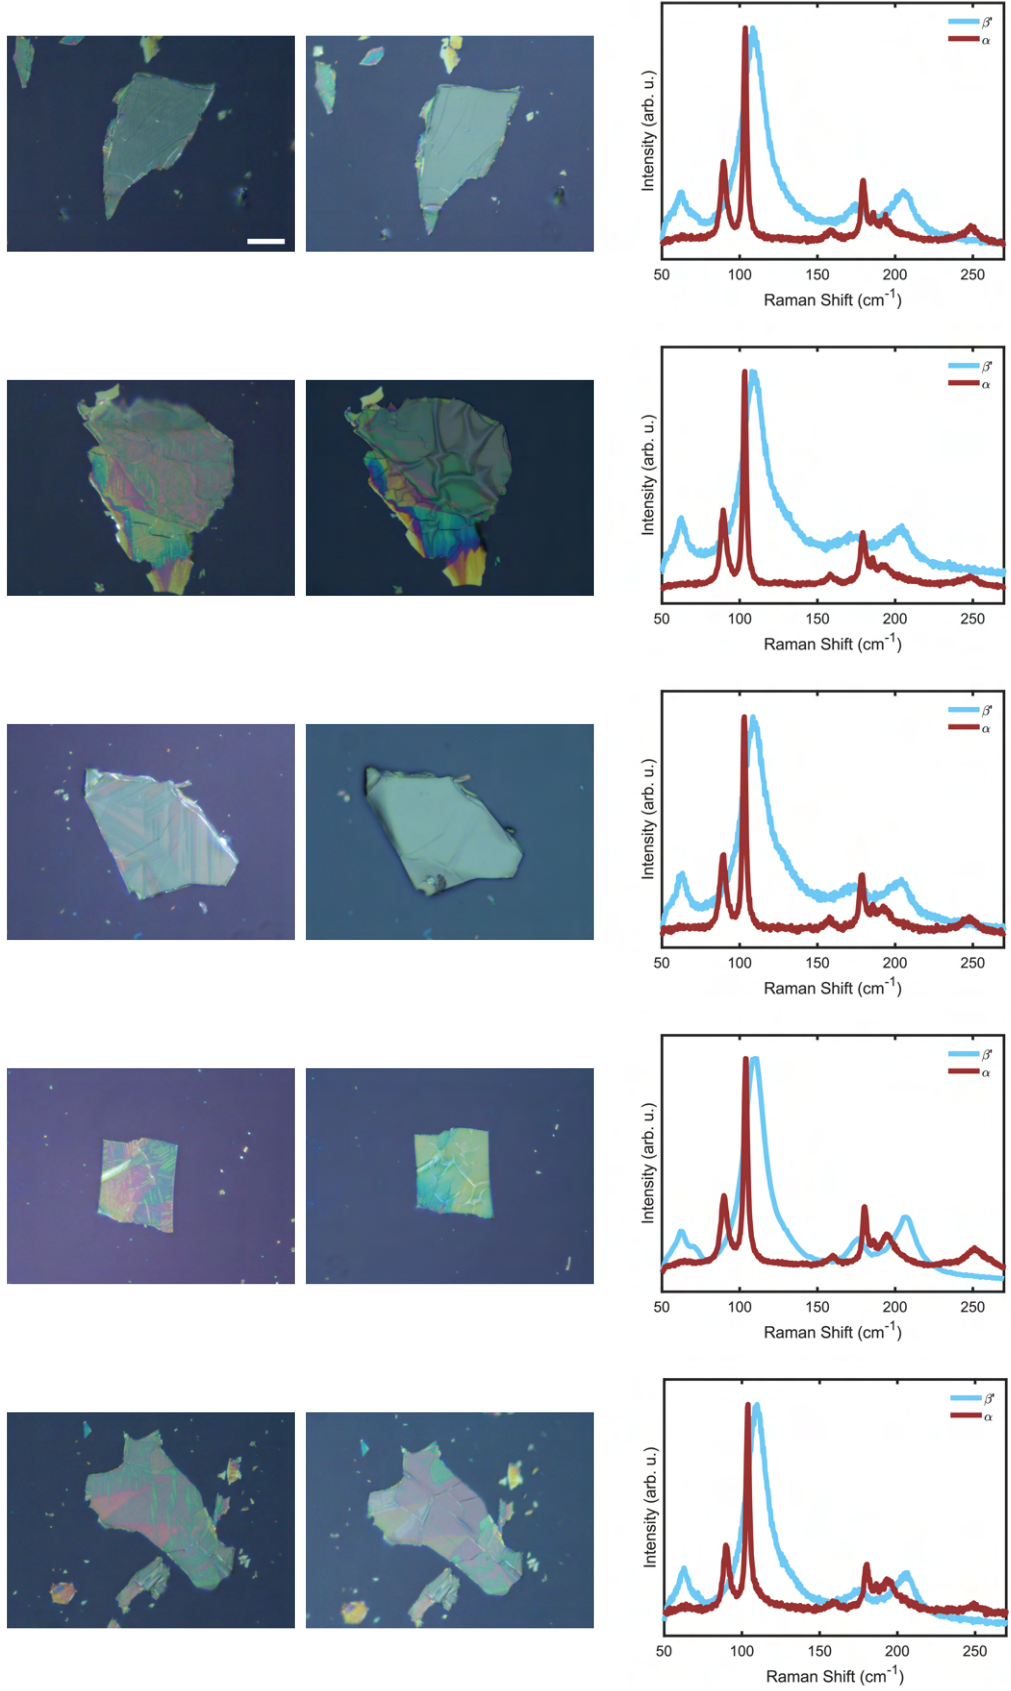

FIG. S5. Cross-polarized Optical images and Raman spectra of flakes on  $\text{SiO}_2$  substrate before and after wrinkling phase transition. Scale bars: 20  $\mu\text{m}$ .

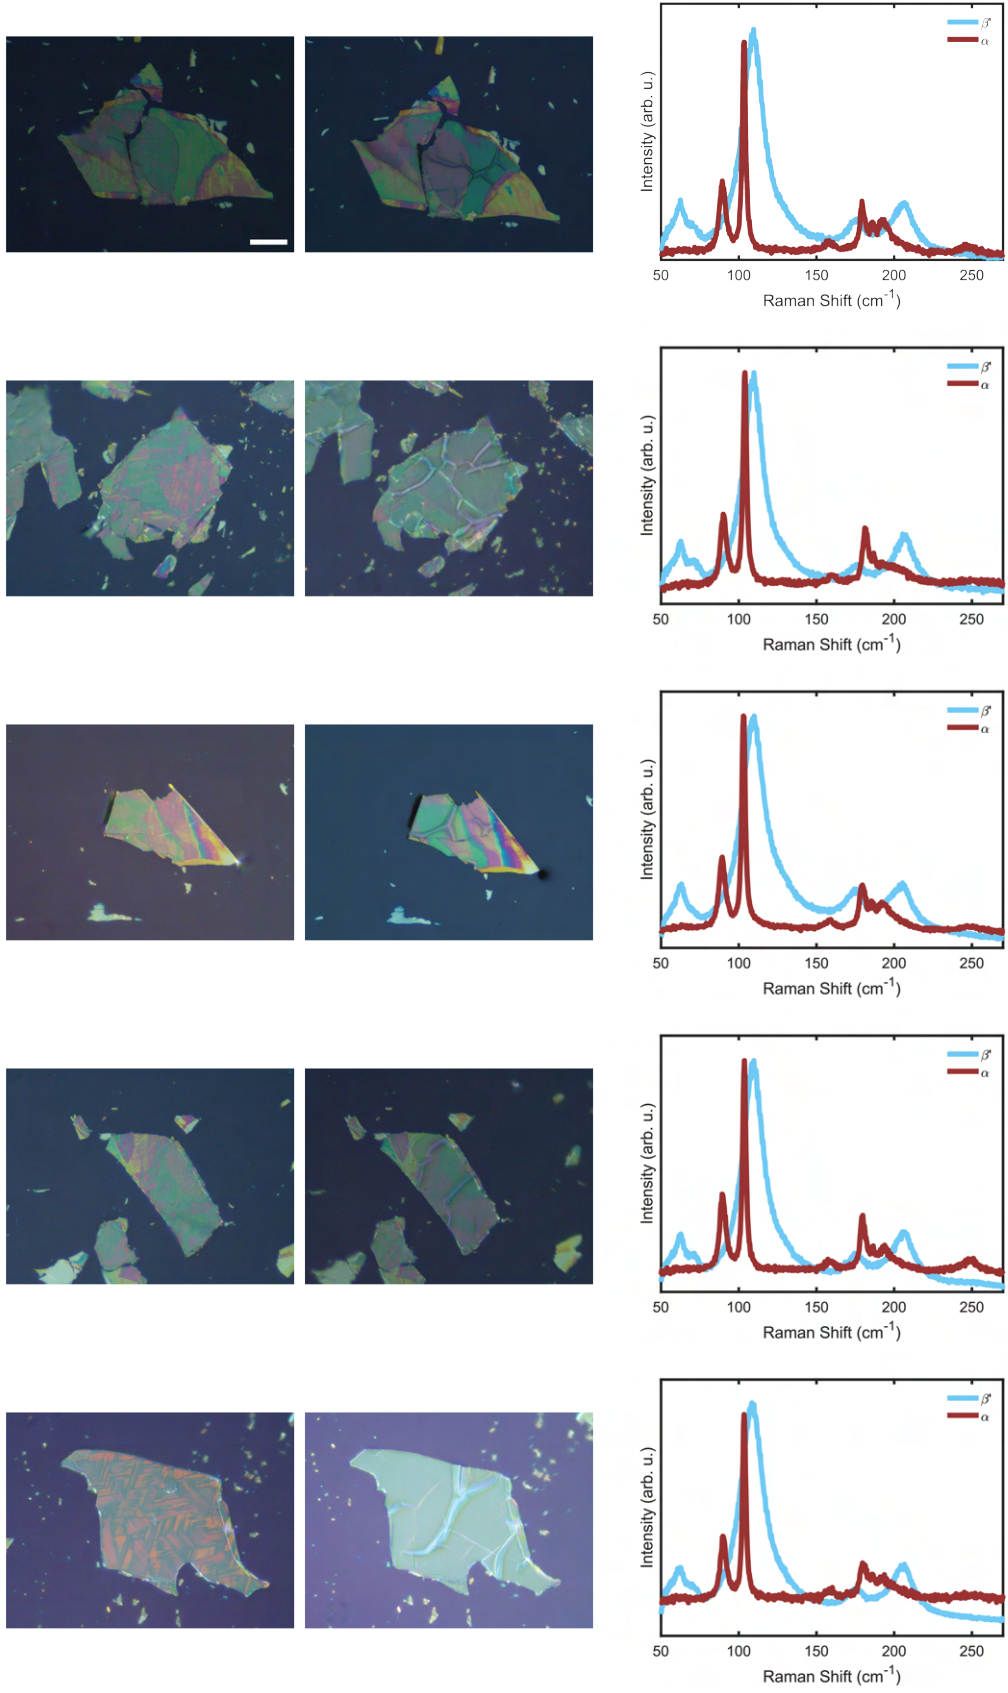

FIG. S6. Additional cross-polarized Optical images and Raman spectra of flakes on SiO<sub>2</sub> substrate before and after wrinkling phase transition. Scale bars: 20 μm.

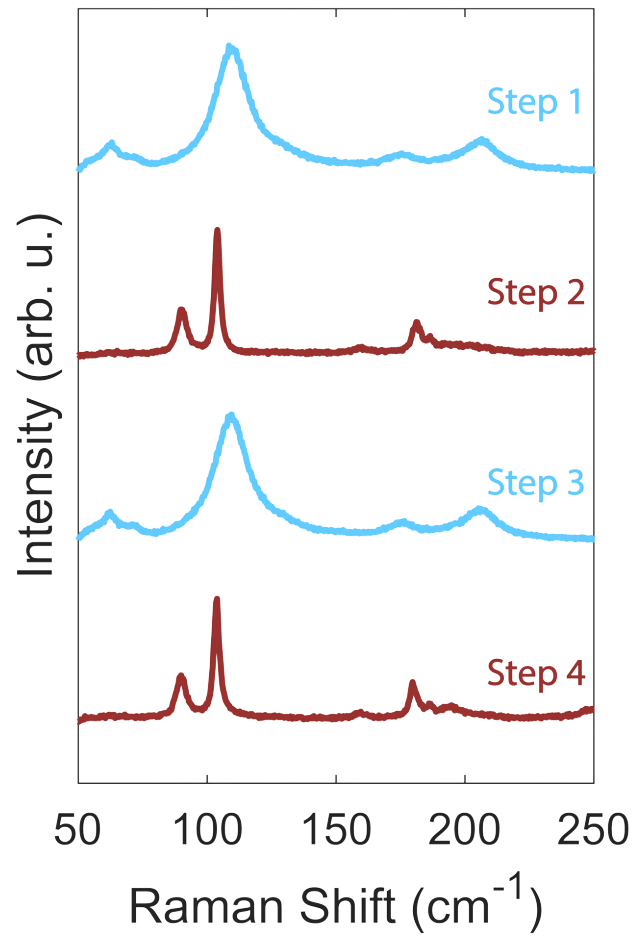

FIG. S7. Raman spectra associated with each step in the phase cycling process shown in Figure 2 of the main text. Blue lines are  $\beta'$  and red are  $\alpha$  phase.

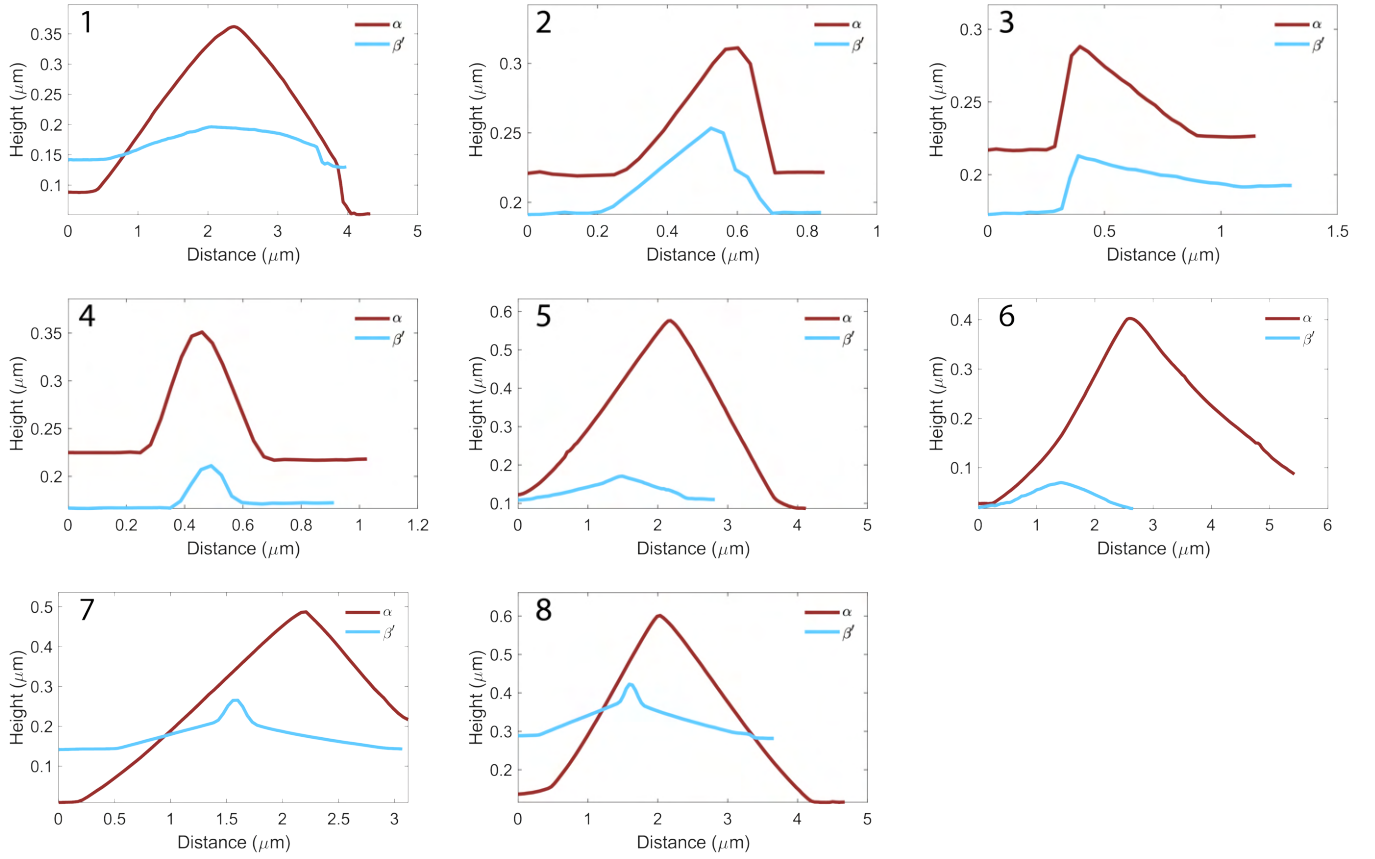

FIG. S8. Profiles along wrinkles corresponding to the height data in Figure 2(E) in the main text. Red traces are  $\alpha$  phase after wrinkling and blue traces are profiles along the same wrinkle after annealing.

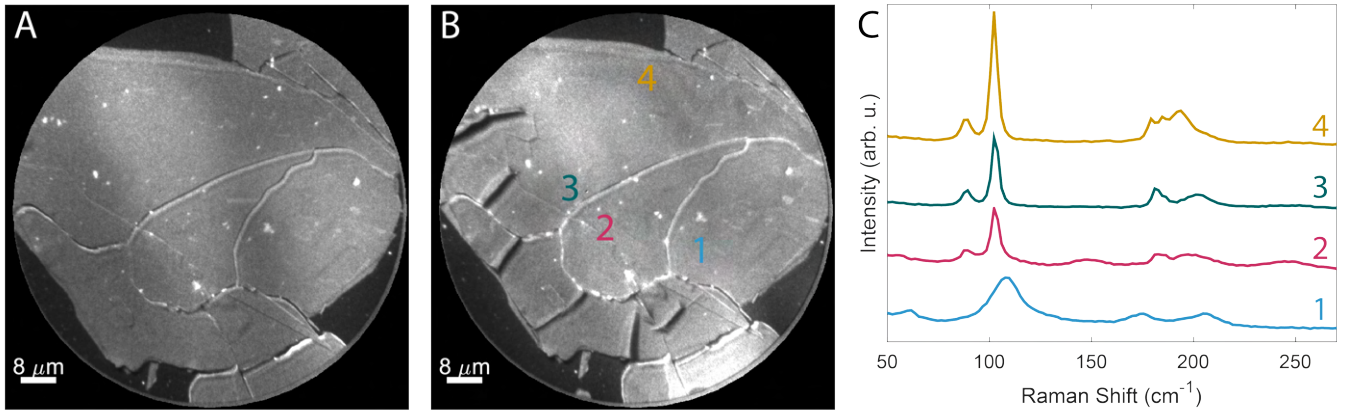

FIG. S9. (A) Static PEEM image of pristine  $\beta'$ - $\text{In}_2\text{Se}_3$  flake with several topographical features. (B) Wrinkled flake after laser exposure ( $h\nu = 3.1\text{eV}$ , Beam spot =  $20 \times 15\mu\text{m}$ , fluence  $\approx 3000\mu\text{J}/\text{cm}^2$ ). The beam spot was smaller than the flake so the wrinkling could be focused at a only a small location. Several wrinkling steps were conducted with the beam at various locations around the flake. (C) Raman spectra at various location. Region 1 remain in  $\beta'$  phase due to the physical boundary that prevented it from converting. The rest of the flake became  $\alpha$  phase. We attribute the additional peaks observed in region 2 at about  $150\text{cm}^{-1}$  and  $240\text{cm}^{-1}$  to a thin film of  $\gamma$ - $\text{In}_2\text{Se}_3$  forming on top of the flake. In some other sample we also observe this effect on  $\beta'$  phase flakes that did not wrinkle and convert to  $\alpha$ - $\text{In}_2\text{Se}_3$ . Spectra were collected with  $\lambda = 532\text{ nm}$  excitation.

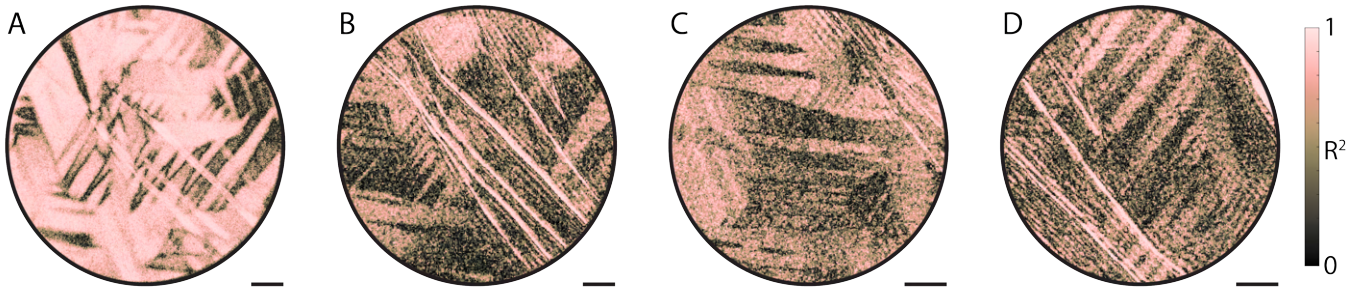

FIG. S10. Maps of  $R^2$  for the pixel-by-pixel fitting in the polarization dependent measurements shown in Figure 4 in the main text and Figure S11. Scalebars are  $2\mu m$ .

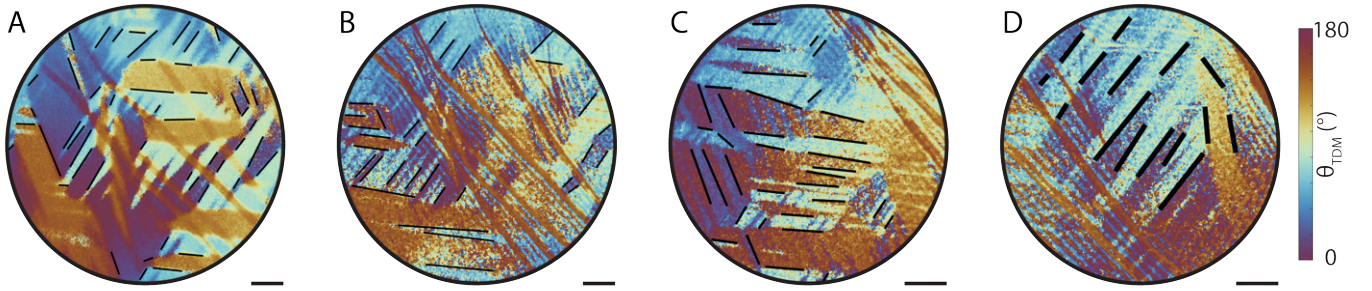

FIG. S11. Domain wall measurements included in the histogram of domain wall orientations in the histogram in Figure 4(C) in the main text. Since a slightly different field of view was used in the final step of the phase cycling process, a second measurement was conducted on the other side of the flake to verify that the lattice vector orientation was conserved on both sides of the step edge, shown in panel (D). Domain walls from both (C) and (D) are included in the histogram. Scalebars are  $2\mu m$ .

## I. SUPPLEMENTARY MOVIE

Supplemental Movie 1 (In2Se3Movie.mp4): Movie of the laser wrinkling experiment. Caption indicates total cumulative laser exposure time. Power = 57.7 mW, Beam spot  $\approx 1 \times 10^5 \mu\text{m}^2$ .
